# Supplementary material for: Improving Proactive AI Assistance with Hierarchical Procedural Understanding
Source: arXiv:2610.06505 source file (2026-10-06)
Supplement: Supplementary file 1 [file 7_supp.tex]

% Appendix-only automatic table of contents. Keep the ICLR style unchanged.
\clearpage
\makeatletter
\let\HUPPAoriginaladdcontentsline\addcontentsline
\renewcommand{\addcontentsline}[3]{%
  \HUPPAoriginaladdcontentsline{#1}{#2}{#3}%
  \def\HUPPAtocfile{#1}%
  \def\HUPPAmaintoc{toc}%
  \ifx\HUPPAtocfile\HUPPAmaintoc
    \addtocontents{atoc}{%
      \protect\contentsline{#2}{#3}{\thepage}{\@currentHref}%
      \protected@file@percent}%
  \fi
}
\phantomsection
\pdfbookmark[0]{Appendices}{appendix.contents}
\begingroup
  \setcounter{tocdepth}{2}
  \setlength{\parskip}{0pt}
  \noindent{\huge\bfseries Appendices\par}
  \vspace{1.5em}
  % Increase TOC line spacing only; preserve the larger gaps before sections.
  % The surrounding group restores the body-text spacing after the TOC.
  \renewcommand{\baselinestretch}{1.5}
  \normalsize
  \@starttoc{atoc}
\endgroup
\makeatother
\clearpage

% Active Appendix: one source file for each section A--I.
% Section/subsection labels use the lowercase heading text, with spaces.
% The TOC is generated from active headings; archived material is excluded.
\input{sec/appendix/a_dataset_specification}
\input{sec/appendix/b_construction_details}
\input{sec/appendix/dataset_storyboards}
\input{sec/appendix/c_annotation_quality}
\input{sec/appendix/d_evaluation_details}
\input{sec/appendix/e_metrics}
\input{sec/appendix/f_additional_quantitative_results}
\input{sec/appendix/g_qualitative_results}
\input{sec/appendix/h_limitations}

\let\addcontentsline\HUPPAoriginaladdcontentsline

% Historical results and the previous HoloAssist-only protocol are preserved
% separately and intentionally NOT included in the current Appendix.
% Archive entry point (enable only when explicitly requested):
% \input{sec/archive/previous_results}
%
% Earlier source copies remain for reference and must not be loaded together
% with their active replacements above:
% sec/appendix/d_evaluation_protocol.tex (also contains earlier writing notes)
% sec/appendix/e_additional_results.tex (also contains commented archives)
% sec/appendix/f_qualitative_results.tex
% sec/appendix/g_limitations_release.tex
%
% The older sec/8_api_quality.tex is also not included; the active quality
% review is sec/appendix/c_annotation_quality.tex. Do not load both copies.
