# Supplementary material for: Improving Proactive AI Assistance with Hierarchical Procedural Understanding
Source: arXiv:2610.06505 source file (2026-10-06)
Supplement: Supplementary file 2 [file a_dataset_specification.tex]

\section{More Details of ProactiveCoach-Instruct and ProactiveCoachBench}
\label{more details of huppa}
Our dataset contains 11,119 samples constructed from 7,232 first-person videos across eight source datasets.
As shown in Table~\ref{tab:hipropa-stats}, 10,007 samples are used for ProactiveCoach-Instruct and 1,112 samples for ProactiveCoachBench.
Samples from the same video are assigned to the same split.
As shown in Figure~\ref{fig:hipropa-duration}, the average sample duration is 7.8 minutes and the median is 8.8 minutes, with durations ranging from 40 seconds to 18 minutes.
The total duration is 1,452.1 hours.
Each sample includes the corresponding events, level-specific guidance, and guidance times.
The data contain 582,084 guidance targets in total: 46,074 at the phase level, 154,507 at the step level, and 381,503 at the action level.
On average, each sample contains 4.14 phases, with 3.35 steps per phase and 2.47 actions per step.

\begin{figure}[H]
\centering
\begin{minipage}[t]{0.48\linewidth}
    \vspace{0pt}
    \centering
    \includegraphics[width=\linewidth]{figs/hipropa_durations.pdf}
    \captionsetup{font=small}
    \caption{Sample duration distribution.}
    \label{fig:hipropa-duration}
\end{minipage}\hfill
\begin{minipage}[t]{0.48\linewidth}
    \vspace{0pt}
    \centering
    \small
    \setlength{\tabcolsep}{3pt}
    \begin{adjustbox}{max width=\linewidth}
    \begin{tabular}{lrrr}
        \toprule
        Property & Train & Test & Total \\
        \midrule
        Samples
            & 10{,}007 & 1{,}112 & 11{,}119 \\
        Unique video files
            & 6{,}517 & 715 & 7{,}232 \\
        Duration (hours)
            & 1{,}306.9 & 145.1 & 1{,}452.1 \\
        \bottomrule
    \end{tabular}
    \end{adjustbox}
    \captionsetup{font=small}
    \captionof{table}{Dataset split statistics.}
    \label{tab:hipropa-stats}
\end{minipage}
\end{figure}
