# Supplementary material for: Improving Proactive AI Assistance with Hierarchical Procedural Understanding
Source: arXiv:2610.06505 source file (2026-10-06)
Supplement: Supplementary file 3 [file b_construction_details.tex]

\begingroup
\raggedbottom
\section{Dataset Construction Details}
\label{dataset construction details}
We construct ProactiveCoach-Instruct and ProactiveCoachBench following the pipeline described in Sec.~\ref{construction pipeline} and Figure~\ref{fig:dataset-construction}: procedural data curation, procedure hierarchy construction, and proactive guidance generation.
We provide prompt details for each stage.
We use Gemini 2.5 Flash for video-grounded recaptioning, GPT-4.1-mini for the remaining generation and filtering steps, and GPT-4.1-mini for hierarchy checking and refinement.
Guide timing assignment follows a rule-based procedure.
\definecolor{hipropapromptblue}{HTML}{236AA0}
\definecolor{hipropapromptgreen}{HTML}{BE7546}
\definecolor{hipropapromptpurple}{HTML}{548249}
\newtcolorbox{hipropaprompt}[2]{
  colback=#1!3!white,colframe=#1,colbacktitle=#1,coltitle=white,
  title={#2},fonttitle=\small\bfseries,fontupper=\footnotesize,
  boxrule=0.5pt,arc=2mm,left=2mm,right=2mm,top=1.5mm,bottom=1.5mm,
  before skip=0pt,after skip=0pt}
\newcommand{\hipropainput}[1]{\texttt{\{#1\}}}

\subsection{Procedural Data Curation}
\label{procedural data curation}
Figures~\ref{fig:construction-prompt-1-1} and~\ref{fig:construction-prompt-1-2} present the prompts for procedural video selection and video-grounded recaptioning, respectively.

\begin{figure}[H]
\centering
\captionsetup{skip=4pt}
\begin{hipropaprompt}{hipropapromptblue}{Procedural Video Selection (Stage 1-1)}
\textbf{System.}\par
You select videos for goal-directed procedural assistance.\par\smallskip
\textbf{Input.}\par
\texttt{video\_metadata} and \texttt{source\_captions}.\par\smallskip
\textbf{Requirements.}\par
1. Assess whether the ordered captions describe a clear task goal and a recognizable outcome.\par
2. Score goal clarity, coverage of key operations, and logical order from 1 to 10. Repeated motions do not count as distinct procedural stages.\par
3. Return an overall suitability score and a short evidence-based reason. Do not assume missing operations occurred.\par
4. Based on these scores and reasoning, decide whether the video should be selected for procedural assistance. \par
\smallskip\textbf{Output.}\par
A JSON object with \texttt{goal\_guess}, \texttt{goal\_score}, \texttt{coverage}, \texttt{order}, \texttt{overall\_score}, \texttt{reasoning}, and \texttt{selected}.\par\smallskip
\end{hipropaprompt}
\vspace{0.3cm}
\caption{Prompt for Procedural Video Selection.}
\label{fig:construction-prompt-1-1}
\end{figure}

\begin{figure}[H]
\centering
\captionsetup{skip=4pt}
\begin{hipropaprompt}{hipropapromptblue}{Video-grounded Recaptioning (Stage 1-2)}
\textbf{System.}\par
You produce video-grounded captions for an egocentric procedural video.\par\smallskip
\textbf{Input.}\par
\texttt{video\_clip}, \texttt{clip\_metadata}, and \texttt{source\_captions}.\par\smallskip
\textbf{Requirements.}\par
1. Use source captions as references and verify each caption against the video. Preserve supported content, correct inaccurate descriptions, supplement visible omissions, and reject unsupported captions.\par
2. Make the caption granularity consistent across source datasets. Each caption should describe a single observable fine-grained manipulation.\par
3. Align each caption's event interval with the corresponding event observed in the video.\par
4. Describe only actions, objects, and state changes that are supported by the video. Do not infer unobserved actions or states. Use English descriptions.\par
\smallskip\textbf{Output.}\par
A JSON object with \texttt{captions}. Each caption contains \texttt{id}, \texttt{description}, \texttt{object}, \texttt{state\_change}, \texttt{event\_interval}, and its source caption reference.
\texttt{object} and \texttt{state\_change} may be null when they are not clearly observable in the video.
Newly added captions may have no source caption reference.\par\smallskip
\end{hipropaprompt}
\vspace{0.3cm}
\caption{Prompt for Video-grounded Recaptioning.}
\label{fig:construction-prompt-1-2}
\end{figure}

\subsection{Procedure Hierarchy Construction}
\label{procedure hierarchy construction}
Figures~\ref{fig:construction-prompt-2-1}, \ref{fig:construction-prompt-2-2}, and~\ref{fig:construction-prompt-2-3} present the prompts for goal-relevant annotation filtering, hierarchical procedure construction, and hierarchy checking and refinement, respectively.

\begin{figure}[H]
\centering
\captionsetup{skip=4pt}
\begin{hipropaprompt}{hipropapromptgreen}{Goal-Relevant Annotation Filtering (Stage 2-1)}
\textbf{System.}\par
You select annotations that contribute to the supplied task goal. Output only JSON.\par\smallskip
\textbf{Input.}\par
\texttt{task\_goal} and \texttt{video\_grounded\_annotations}.\par\smallskip
\textbf{Requirements.}\par
1. Judge each annotation in the context of the task goal and surrounding annotations. Keep annotations that directly contribute to the task or support a necessary operation.\par
2. Retain preparation and supporting events, such as fetching an ingredient, measuring, or opening a container, when they serve the goal. Repeated events are not automatically irrelevant.\par
3. Exclude activity unrelated to the task goal, such as an unrelated conversation or camera adjustment. Do not reject an annotation merely because it does not yet fit a Step.\par
4. Preserve annotation IDs, descriptions, objects, state changes, and event intervals. Give an evidence-based reason for exclusions; do not invent missing operations.\par
\smallskip\textbf{Output.}\par
A JSON object with \texttt{retained\_ids} and \texttt{excluded}; each excluded entry contains \texttt{annotation\_id} and \texttt{reason}. Account for every input annotation exactly once.\par\smallskip
\end{hipropaprompt}
\vspace{0.3cm}
\caption{Prompt for Goal-Relevant Annotation Filtering.}
\label{fig:construction-prompt-2-1}
\end{figure}

\begin{figure}[H]
\centering
\captionsetup{skip=4pt}
\begin{hipropaprompt}{hipropapromptgreen}{Hierarchical Procedure Construction (Stage 2-2)}
\textbf{System.}\par
You organize observed activity into a Phase--Step--Action hierarchy.\par\smallskip
\textbf{Input.}\par
\texttt{task\_goal}, \texttt{retained\_annotations}, and \texttt{review\_feedback} (if any).\par\smallskip
\textbf{Requirements.}\par
1. Consolidate the retained annotations into observable Actions that are meaningful to guide independently. Use their descriptions, objects, state changes, and event intervals to determine which annotations belong to the same Action. Merge annotations that describe the same event while preserving distinct events, and set each Action interval to cover the event intervals of its annotations.\par
2. Group Actions that together form a procedural task into a Step, and group Steps that together achieve an intermediate goal into a Phase. Define levels by procedural scope, not sentence length.\par
3. Set each Step interval to cover its Action intervals, and each Phase interval to cover its Step intervals.\par
4. Each Action belongs to one Step and each Step to one Phase. Descriptions at a higher level must express the collective scope of the lower-level units they contain. Avoid a Phase--Step--Action chain that merely renames the same operation; do not create additional Actions or Steps only to increase branching.\par
5. When review feedback is supplied, reconstruct the affected groups using the retained annotations and preserve valid assignments. Return explicit Phase--Step, Step--Action, and annotation references.\par
\smallskip\textbf{Output.}\par
A JSON object with \texttt{phases}, \texttt{steps}, and \texttt{actions}. Each unit contains \texttt{id}, \texttt{description}, \texttt{event\_interval}, and \texttt{annotation\_ids}. Each Step contains its \texttt{phase\_id}, and each Action contains its \texttt{step\_id}.\par\smallskip
\end{hipropaprompt}
\vspace{0.3cm}
\caption{Prompt for Hierarchical Procedure Construction.}
\label{fig:construction-prompt-2-2}
\end{figure}

\begin{figure}[H]
\centering
\captionsetup{skip=4pt}
\begin{hipropaprompt}{hipropapromptgreen}{Hierarchy Checking and Refinement (Stage 2-3)}
\textbf{System.}\par
You review the scope and evidence support of a proposed procedural hierarchy.\par\smallskip
\textbf{Input.}\par
\texttt{task\_goal}, \texttt{retained\_annotations}, and \texttt{candidate\_hierarchy}.\par\smallskip
\textbf{Requirements.}\par
1. Check whether each lower-level unit contributes to the higher-level unit that contains it. Use the retained annotation descriptions, objects, state changes, and event intervals as evidence, and check whether relevant observed operations are missing or duplicated.\par
2. Flag higher-level units whose scope is not supported by the lower-level units they contain, as well as Phase--Step--Action chains that express the same operation across levels. A lower-level unit count alone is not sufficient; inspect the actual procedural scope.\par
3. Check Phase--Step and Step--Action references, chronological order, and whether each higher-level event interval covers the event intervals of the lower-level units it contains. Separate temporal errors from semantic grouping errors.\par
4. Return evidence-based reconstruction feedback for affected units to 2-2. Preserve valid groups and do not invent unobserved operations.\par
\smallskip\textbf{Output.}\par
A JSON object with \texttt{passed}, \texttt{issues}, and \texttt{reconstruction\_feedback}. Each issue identifies the affected unit, issue type, annotation IDs, and requested correction.\par\smallskip
\end{hipropaprompt}
\vspace{0.3cm}
\caption{Prompt for Hierarchy Checking and Refinement.}
\label{fig:construction-prompt-2-3}
\end{figure}

\subsection{Proactive Guidance Generation}
\label{proactive guidance generation}
Figure~\ref{fig:construction-prompt-3-1} presents the prompt for level-specific guidance generation.
In Guide Timing Assignment (Stage 3-2), guidance timing is determined independently at the Phase, Step, and Action levels.
Within the same level, the next guidance is assigned to the first frame after the current event ends.
The first guidance at each level is assigned to the first frame of the video.
When guidance from multiple levels is assigned to the same frame, we combine it into a single \texttt{<response>} in Phase, Step, and Action order.
If no guidance is assigned at any level, the frame is labeled \texttt{<silent>}.


\begin{figure}[h]
\centering
\captionsetup{skip=4pt}
\begin{hipropaprompt}{hipropapromptpurple}{Level-Specific Guidance Generation (Stage 3-1)}
\textbf{System.}\par
You write proactive instructions that match the scope of each Phase, Step, and Action.\par\smallskip
\textbf{Input.}\par
\texttt{task\_goal}, \texttt{hierarchy\_units}, and \texttt{supporting\_annotations}.\par\smallskip
\textbf{Requirements.}\par
1. Use the task goal, hierarchy context, and supporting annotations to write an actionable imperative instruction in English.\par
2. Phase guidance conveys an intermediate goal; Step guidance conveys a procedural task; Action guidance conveys a concrete manipulation.\par
3. Do not describe a higher-level task using only its first lower-level operation. Do not include content from another unit or add unsupported details. Avoid filler.\par
4. Check each instruction against its corresponding Phase, Step, or Action and supporting annotations, correcting inaccurate objects, unsupported details, or scope mismatches. Preserve the supplied unit IDs. Generate content only; timing is assigned separately.\par
\smallskip\textbf{Output.}\par
A JSON object with \texttt{guidance}; each entry contains \texttt{unit\_id}, \texttt{level}, and \texttt{instruction}.\par\smallskip
\end{hipropaprompt}
\vspace{0.3cm}
\caption{Prompt for Level-Specific Guidance Generation.}
\label{fig:construction-prompt-3-1}
\end{figure}
\endgroup
