# Supplementary material for: Improving Proactive AI Assistance with Hierarchical Procedural Understanding
Source: arXiv:2610.06505 source file (2026-10-06)
Supplement: Supplementary file 4 [file c_annotation_quality.tex]

\section{Details of Quality Review}
\label{details of quality review}

We conduct a human quality review on 50 test examples at the phase, step, and action levels using four criteria: \textit{video alignment}, \textit{hierarchical coverage}, \textit{goal relevance}, and \textit{guidance quality}.
Figure~\ref{fig:human-review-ui} shows the interface used for the evaluation.

\begin{figure}[h]
\centering
\includegraphics[
width=\linewidth,
height=.82\textheight,
keepaspectratio]{figs/fig14.pdf}
\caption{
Human quality review interface.
Reviewers inspect the task video and its hierarchical annotations at the phase, step, and action levels and evaluate them using four criteria: video alignment, hierarchical coverage, goal relevance, and guidance quality.
}
\label{fig:human-review-ui}
\end{figure}

\textit{Video alignment} evaluates whether the annotated content, temporal spans, and guidance timing are consistent with the observed video.
Guidance may be provided before the next execution begins.
However, guidance that is provided excessively early or late, or unnecessarily repeats a completed execution, is rated lower.
The scores are 4.05, 4.14, and 3.80 for the phase, step, and action levels, respectively, showing that the annotations generally align well with the video progress.

\textit{Hierarchical coverage} evaluates whether lower-level executions sufficiently cover the content required by the higher-level procedure.
We examine whether the phases cover the activities needed to achieve the goal, the steps cover each phase, and the actions cover each step, focusing on whether any essential execution is missing.
The scores are 4.35, 4.50, and 4.48, respectively, indicating strong coverage across all levels.

\textit{Goal relevance} evaluates whether the selected executions and guidance contribute to achieving the task goal.
Preparatory, safety-related, and recovery events that are necessary to achieve the task goal are considered relevant, whereas events unrelated to the goal are rated lower.
The scores are 4.48, 4.41, and 4.39, respectively, showing high goal relevance across all levels.

\textit{Guidance quality} evaluates whether each guidance sentence clearly and accurately describes what the user should do at the corresponding level.
Lower scores are assigned when the guidance is unclear, difficult to follow, or does not match the intended level of detail.
The scores are 4.37, 4.16, and 4.16, respectively, indicating that the generated guidance is generally clear and appropriate for each level.
