# Supplementary material for: Improving Proactive AI Assistance with Hierarchical Procedural Understanding
Source: arXiv:2610.06505 source file (2026-10-06)
Supplement: Supplementary file 5 [file d_detailed_metrics.tex]

% Mirrors main-text Tables 2--5; values come from the same evaluation runs.
\providecommand{\TSnoft}{}
\providecommand{\TSyesft}{\ensuremath{\checkmark}}
As discussed in Section~\ref{details of metrics}, our evaluation metrics are computed from sPrecision, sRecall, Response F1, and Silence F1.
Tables~\ref{tab:details_main_results}--\ref{tab:details_joint_guidance} report these four metrics in detail.
Table~\ref{tab:details_main_results} shows that our method achieves a better balance between Response F1 and Silence F1, together with substantial gains in sPrecision.
Tables~\ref{tab:details_multilevel_supervision}--\ref{tab:details_training_levels} further show the effects of hierarchical supervision and different supervision levels.
Table~\ref{tab:details_joint_guidance} provides the results for zero-shot and fine-tuned multi-level guidance.
\vspace{-0.1cm}

% As discussed in Section~\ref{details of metrics}, our metrics used in evaluation are extracted from sPrecision, sRecall, Response F1, and Silence F1 metrics. Tables~\ref{tab:details_main_results}--\ref{} shows the performance of these metrics.
% Table~\ref{tab:details_main_results} shows that our method achieves a better balance between Response F1 and Silence F1, together with large gains in sPrecision.
% Also, Table~\ref{tab:details_multilevel_supervisions}--\ref{, tab:details_training_level} demonstrates improvements under multi-level and hierarchical supervision.
% , \red{while Table~11 shows substantial gains across all four metrics for guidance-level adaptation.}

\begin{comment}
\noindent The following tables report sPrecision, sRecall, Response F1, and Silence F1
for the same models, settings, and evaluated samples as Tables~\ref{tab:main_results}--\ref{tab:guidance-level-adaptation}.
Notation follows the corresponding main-text tables.
All metrics are percentages; sPrecision and sRecall are record-wise averages.
\end{comment}

\begin{table*}[h]
  \renewcommand{\cellcolor}[1]{} % Plain result cells; retain status markup for automatic updates.
  \centering
  \scriptsize
  \setlength{\tabcolsep}{2.0pt}
  \renewcommand{\arraystretch}{1.30}
  \begin{adjustbox}{max width=\textwidth}
  \begin{tabular}{l|c|cccc|cccc|cccc|cccc}
    \noalign{\hrule height 1pt}
    \multirow{3}{*}{Model} & \multirow{3}{*}{Ours} & \multicolumn{12}{c|}{ProactiveCoachBench} & \multicolumn{4}{c}{EgoProactive} \\
    \cline{3-14}\cline{15-18}
    & & \multicolumn{4}{c|}{Phase} & \multicolumn{4}{c|}{Step} & \multicolumn{4}{c|}{Action} & \multicolumn{4}{c}{Step} \\
    \cline{3-6}\cline{7-10}\cline{11-14}\cline{15-18}
    & & sPrecision & sRecall & Response F1 & Silence F1 & sPrecision & sRecall & Response F1 & Silence F1 & sPrecision & sRecall & Response F1 & Silence F1 & sPrecision & sRecall & Response F1 & Silence F1 \\
    \noalign{\hrule height 0.6pt}
    \multicolumn{18}{c}{Proprietary Frontier Models}  \\ \hline
    Gemini 3 Flash Preview & \TSnoft & \cellcolor{gray!15}53.05 & \cellcolor{gray!15}39.68 & \cellcolor{gray!15}66.25 & \cellcolor{gray!15}74.73 & \cellcolor{gray!15}41.47 & \cellcolor{gray!15}44.11 & \cellcolor{gray!15}59.66 & \cellcolor{gray!15}58.35 & \cellcolor{gray!15}39.92 & \cellcolor{gray!15}54.68 & \cellcolor{gray!15}65.26 & \cellcolor{gray!15}50.59 & \cellcolor{gray!15}52.05 & \cellcolor{gray!15}33.04 & \cellcolor{gray!15}60.74 & \cellcolor{gray!15}68.91 \\ % DETAIL_SOURCE METRICS_CELL anchor2/phase-gemini3flash/phase anchor2/family-gemini/step anchor2/action-gemini3flash/action anchor3/family-gemini/step
    Claude Haiku 4.5 & \TSnoft & \cellcolor{gray!15}35.41 & \cellcolor{gray!15}60.87 & \cellcolor{gray!15}64.90 & \cellcolor{gray!15}11.82 & \cellcolor{gray!15}32.05 & \cellcolor{gray!15}62.78 & \cellcolor{gray!15}65.77 & \cellcolor{gray!15}7.73 & \cellcolor{gray!15}32.12 & \cellcolor{gray!15}62.96 & \cellcolor{gray!15}66.14 & \cellcolor{gray!15}8.64 & \cellcolor{gray!15}35.13 & \cellcolor{gray!15}46.02 & \cellcolor{gray!15}63.84 & \cellcolor{gray!15}43.39 \\ % DETAIL_SOURCE METRICS_CELL anchor2/phase-haiku45/phase anchor2/family-claude/step anchor2/action-haiku45/action anchor3/family-claude/step
    GPT‑5.4 mini & \TSnoft & \cellcolor{gray!15}33.06 & \cellcolor{gray!15}38.50 & \cellcolor{gray!15}55.81 & \cellcolor{gray!15}44.84 & \cellcolor{gray!15}33.41 & \cellcolor{gray!15}36.17 & \cellcolor{gray!15}54.25 & \cellcolor{gray!15}48.33 & \cellcolor{gray!15}37.06 & \cellcolor{gray!15}35.83 & \cellcolor{gray!15}53.94 & \cellcolor{gray!15}53.80 & \cellcolor{gray!15}39.05 & \cellcolor{gray!15}43.05 & \cellcolor{gray!15}61.03 & \cellcolor{gray!15}47.08 \\ % DETAIL_SOURCE METRICS_CELL anchor2/phase-gpt54mini/phase anchor2/family-gpt/step anchor2/action-gpt54mini/action anchor3/family-gpt/step
    \noalign{\hrule height 0.6pt}
    \multicolumn{18}{c}{Guidance Assistant Models} \\ \hline
    ProAssist-8B & \TSnoft & \cellcolor{gray!15}21.55 & \cellcolor{gray!15}8.22 & \cellcolor{gray!15}22.33 & \cellcolor{gray!15}67.63 & \cellcolor{gray!15}28.19 & \cellcolor{gray!15}6.28 & \cellcolor{gray!15}17.14 & \cellcolor{gray!15}66.33 & \cellcolor{gray!15}37.18 & \cellcolor{gray!15}6.28 & \cellcolor{gray!15}14.48 & \cellcolor{gray!15}66.17 & \cellcolor{gray!15}19.18 & \cellcolor{gray!15}3.83 & \cellcolor{gray!15}9.64 & \cellcolor{gray!15}63.02 \\ % DETAIL_SOURCE METRICS_CELL anchor2/proassist-i1-subset10/phase anchor2/proassist-i1-subset10/step anchor2/proassist-i1-subset10/action anchor3/proassist-i1-subset10/step
    \noalign{\hrule height 0.6pt}
    \multicolumn{18}{c}{Streaming Models} \\ \hline
    VideoLLM-Online & \TSnoft & \cellcolor{gray!15}1.06 & \cellcolor{gray!15}0.30 & \cellcolor{gray!15}1.21 & \cellcolor{gray!15}66.72 & \cellcolor{gray!15}2.16 & \cellcolor{gray!15}0.18 & \cellcolor{gray!15}0.63 & \cellcolor{gray!15}66.66 & \cellcolor{gray!15}4.95 & \cellcolor{gray!15}0.18 & \cellcolor{gray!15}0.54 & \cellcolor{gray!15}66.68 & \cellcolor{gray!15}2.17 & \cellcolor{gray!15}0.30 & \cellcolor{gray!15}1.41 & \cellcolor{gray!15}63.27 \\ % DETAIL_SOURCE METRICS_CELL anchor2/videollm-online-recent10/phase anchor2/videollm-online-recent10/step anchor2/videollm-online-recent10/action anchor3/videollm-online-recent10/step
    MMDuet2 & \TSnoft & \cellcolor{gray!15}15.11 & \cellcolor{gray!15}8.73 & \cellcolor{gray!15}27.08 & \cellcolor{gray!15}60.30 & \cellcolor{gray!15}26.16 & \cellcolor{gray!15}19.90 & \cellcolor{gray!15}42.45 & \cellcolor{gray!15}54.85 & \cellcolor{gray!15}27.98 & \cellcolor{gray!15}19.02 & \cellcolor{gray!15}43.16 & \cellcolor{gray!15}56.20 & \cellcolor{gray!15}32.04 & \cellcolor{gray!15}33.28 & \cellcolor{gray!15}52.56 & \cellcolor{gray!15}38.03 \\ % MMDUET_SELECTIVE_DETAIL_ALL mmduet2-selective-available-v1
    VideoChat3-4B & \TSnoft & \cellcolor{gray!15}29.93 & \cellcolor{gray!15}49.55 & \cellcolor{gray!15}60.62 & \cellcolor{gray!15}6.03 & \cellcolor{gray!15}27.80 & \cellcolor{gray!15}50.95 & \cellcolor{gray!15}63.34 & \cellcolor{gray!15}10.37 & \cellcolor{gray!15}29.08 & \cellcolor{gray!15}57.83 & \cellcolor{gray!15}65.61 & \cellcolor{gray!15}4.94 & \cellcolor{gray!15}34.59 & \cellcolor{gray!15}48.71 & \cellcolor{gray!15}61.12 & \cellcolor{gray!15}21.59 \\ % DETAIL_SOURCE FULL_RERUN_VIDEOCHAT3 videochat3-explicit-advice-full-v1
    \noalign{\hrule height 0.6pt}
    \multicolumn{18}{c}{Multimodal Models}
    \\ \hline
    VideoChat-R1.5-7B & \TSnoft & \cellcolor{gray!15}0.09 & \cellcolor{gray!15}0.04 & \cellcolor{gray!15}0.09 & \cellcolor{gray!15}66.67 & \cellcolor{gray!15}0.66 & \cellcolor{gray!15}0.04 & \cellcolor{gray!15}0.23 & \cellcolor{gray!15}66.54 & \cellcolor{gray!15}1.41 & \cellcolor{gray!15}0.06 & \cellcolor{gray!15}0.17 & \cellcolor{gray!15}66.29 & \cellcolor{gray!15}0.62 & \cellcolor{gray!15}0.12 & \cellcolor{gray!15}0.34 & \cellcolor{gray!15}65.02 \\ % DETAIL_SOURCE METRICS_CELL anchor2/vcr15-7b-recent10/phase anchor2/vcr15-7b-recent10/step anchor2/vcr15-7b-recent10/action anchor3/vcr15-7b-recent10/step
    InternVL3-8B & \TSnoft & \cellcolor{gray!15}19.25 & \cellcolor{gray!15}12.23 & \cellcolor{gray!15}34.11 & \cellcolor{gray!15}59.66 & \cellcolor{gray!15}31.73 & \cellcolor{gray!15}24.23 & \cellcolor{gray!15}48.41 & \cellcolor{gray!15}56.15 & \cellcolor{gray!15}37.34 & \cellcolor{gray!15}37.08 & \cellcolor{gray!15}57.48 & \cellcolor{gray!15}52.42 & \cellcolor{gray!15}39.95 & \cellcolor{gray!15}12.63 & \cellcolor{gray!15}23.89 & \cellcolor{gray!15}60.71 \\ % DETAIL_SOURCE METRICS_CELL anchor2/internvl3-8b-recent10/phase anchor2/internvl3-8b-recent10/step anchor2/internvl3-8b-recent10/action anchor3/internvl3-8b-recent10/step
    VideoLLaMA3-7B & \TSnoft & \cellcolor{gray!15}19.75 & \cellcolor{gray!15}15.40 & \cellcolor{gray!15}37.38 & \cellcolor{gray!15}52.87 & \cellcolor{gray!15}28.13 & \cellcolor{gray!15}20.77 & \cellcolor{gray!15}43.33 & \cellcolor{gray!15}54.99 & \cellcolor{gray!15}33.90 & \cellcolor{gray!15}27.95 & \cellcolor{gray!15}48.30 & \cellcolor{gray!15}51.93 & \cellcolor{gray!15}2.88 & \cellcolor{gray!15}0.73 & \cellcolor{gray!15}1.36 & \cellcolor{gray!15}61.27 \\ % DETAIL_SOURCE METRICS_CELL anchor2/videollama3-7b-recent10/phase anchor2/videollama3-7b-recent10/step anchor2/videollama3-7b-recent10/action anchor3/videollama3-7b-recent10/step
    LLaVA-Video-7B & \TSnoft & \cellcolor{gray!15}23.34 & \cellcolor{gray!15}20.20 & \cellcolor{gray!15}43.18 & \cellcolor{gray!15}52.79 & \cellcolor{gray!15}33.51 & \cellcolor{gray!15}32.17 & \cellcolor{gray!15}53.36 & \cellcolor{gray!15}50.00 & \cellcolor{gray!15}39.21 & \cellcolor{gray!15}22.15 & \cellcolor{gray!15}44.54 & \cellcolor{gray!15}59.67 & \cellcolor{gray!15}41.00 & \cellcolor{gray!15}34.89 & \cellcolor{gray!15}48.50 & \cellcolor{gray!15}46.82 \\ % DETAIL_SOURCE METRICS_CELL anchor2/llavavideo-7b-recent10/phase anchor2/llavavideo-7b-recent10/step anchor2/llavavideo-7b-recent10/action anchor3/llavavideo-7b-recent10/step
    Qwen3-VL-32B & \TSnoft & \cellcolor{gray!15}34.84 & \cellcolor{gray!15}56.47 & \cellcolor{gray!15}64.77 & \cellcolor{gray!15}22.89 & \cellcolor{gray!15}29.86 & \cellcolor{gray!15}57.66 & \cellcolor{gray!15}65.45 & \cellcolor{gray!15}8.72 & \cellcolor{gray!15}29.88 & \cellcolor{gray!15}59.25 & \cellcolor{gray!15}66.23 & \cellcolor{gray!15}6.55 & \cellcolor{gray!15}44.01 & \cellcolor{gray!15}28.20 & \cellcolor{gray!15}44.73 & \cellcolor{gray!15}55.47 \\ % DETAIL_SOURCE METRICS_CELL anchor2/q3vl-32b-recent10/phase anchor2/q3vl-32b-recent10/step anchor2/q3vl-32b-recent10/action anchor3/q3vl-32b-recent10/step
    \noalign{\hrule height 0.6pt}
    \multirow{2}{*}{Qwen3-VL-4B} & \TSnoft & \cellcolor{gray!15}29.37 & \cellcolor{gray!15}50.65 & \cellcolor{gray!15}63.88 & \cellcolor{gray!15}10.43 & \cellcolor{gray!15}28.41 & \cellcolor{gray!15}54.59 & \cellcolor{gray!15}65.45 & \cellcolor{gray!15}10.34 & \cellcolor{gray!15}29.04 & \cellcolor{gray!15}56.56 & \cellcolor{gray!15}66.05 & \cellcolor{gray!15}11.68 & \cellcolor{gray!15}35.86 & \cellcolor{gray!15}48.62 & \cellcolor{gray!15}59.59 & \cellcolor{gray!15}21.63 \\ % DETAIL_SOURCE METRICS_CELL anchor2/q3vl-4b-recent10/phase anchor2/q3vl-4b-recent10/step anchor2/q3vl-4b-recent10/action anchor3/q3vl-4b-recent10/step
    {} & \TSyesft & \cellcolor{gray!15}73.95 & \cellcolor{gray!15}44.26 & \cellcolor{gray!15}68.88 & \cellcolor{gray!15}80.38 & \cellcolor{gray!15}59.13 & \cellcolor{gray!15}44.45 & \cellcolor{gray!15}68.04 & \cellcolor{gray!15}75.30 & \cellcolor{gray!15}46.69 & \cellcolor{gray!15}56.37 & \cellcolor{gray!15}68.22 & \cellcolor{gray!15}61.34 & \cellcolor{gray!15}47.66 & \cellcolor{gray!15}31.86 & \cellcolor{gray!15}60.00 & \cellcolor{gray!15}65.69 \\ % DETAIL_SOURCE METRICS_CELL anchor2/ours-q3vl-4b-window10s/phase anchor2/ours-q3vl-4b-window10s/step anchor2/ours-q3vl-4b-window10s/action anchor3/ours-q3vl-4b-window10s/step
    \hline
    \multirow{2}{*}{Qwen3-VL-8B} & \TSnoft & \cellcolor{gray!15}32.56 & \cellcolor{gray!15}59.98 & \cellcolor{gray!15}66.44 & \cellcolor{gray!15}1.37 & \cellcolor{gray!15}29.24 & \cellcolor{gray!15}59.49 & \cellcolor{gray!15}66.47 & \cellcolor{gray!15}1.38 & \cellcolor{gray!15}28.62 & \cellcolor{gray!15}58.92 & \cellcolor{gray!15}66.60 & \cellcolor{gray!15}1.21 & \cellcolor{gray!15}32.94 & \cellcolor{gray!15}59.47 & \cellcolor{gray!15}70.02 & \cellcolor{gray!15}0.09 \\ % DETAIL_SOURCE METRICS_CELL anchor2/q3vl-8b-recent10/phase anchor2/q3vl-8b-recent10/step anchor2/q3vl-8b-recent10/action anchor3/q3vl-8b-recent10/step
    {} & \TSyesft & \cellcolor{gray!15}74.08 & \cellcolor{gray!15}45.87 & \cellcolor{gray!15}71.33 & \cellcolor{gray!15}81.41 & \cellcolor{gray!15}58.70 & \cellcolor{gray!15}46.40 & \cellcolor{gray!15}69.05 & \cellcolor{gray!15}75.12 & \cellcolor{gray!15}46.55 & \cellcolor{gray!15}57.65 & \cellcolor{gray!15}68.05 & \cellcolor{gray!15}60.41 & \cellcolor{gray!15}50.38 & \cellcolor{gray!15}29.57 & \cellcolor{gray!15}58.78 & \cellcolor{gray!15}67.65 \\ % DETAIL_SOURCE METRICS_CELL anchor2/ours-q3vl-8b-window10s/phase anchor2/ours-q3vl-8b-window10s/step anchor2/ours-q3vl-8b-window10s/action anchor3/ours-q3vl-8b-window10s/step
    \hline
    \multirow{2}{*}{Qwen3.5-4B} & \TSnoft & \cellcolor{gray!15}23.00 & \cellcolor{gray!15}18.98 & \cellcolor{gray!15}42.70 & \cellcolor{gray!15}53.64 & \cellcolor{gray!15}28.08 & \cellcolor{gray!15}19.43 & \cellcolor{gray!15}41.67 & \cellcolor{gray!15}57.86 & \cellcolor{gray!15}34.81 & \cellcolor{gray!15}18.77 & \cellcolor{gray!15}38.16 & \cellcolor{gray!15}59.91 & \cellcolor{gray!15}34.34 & \cellcolor{gray!15}10.35 & \cellcolor{gray!15}21.77 & \cellcolor{gray!15}61.80 \\ % DETAIL_SOURCE METRICS_CELL anchor2/qwen-single-level-question-v1/phase anchor2/qwen-single-level-question-v1/step anchor2/qwen-single-level-question-v1/action anchor3/qwen-single-level-question-v1/step
    {} & \TSyesft & \cellcolor{gray!15}72.89 & \cellcolor{gray!15}44.05 & \cellcolor{gray!15}69.86 & \cellcolor{gray!15}80.83 & \cellcolor{gray!15}59.73 & \cellcolor{gray!15}44.23 & \cellcolor{gray!15}69.02 & \cellcolor{gray!15}75.68 & \cellcolor{gray!15}47.18 & \cellcolor{gray!15}57.04 & \cellcolor{gray!15}68.56 & \cellcolor{gray!15}61.15 & \cellcolor{gray!15}48.56 & \cellcolor{gray!15}30.44 & \cellcolor{gray!15}56.32 & \cellcolor{gray!15}64.04 \\ % DETAIL_SOURCE METRICS_CELL anchor2/ours-q35-4b-joint-window10s-20260919/phase anchor2/ours-q35-4b-joint-window10s-20260919/step anchor2/ours-q35-4b-joint-window10s-20260919/action anchor3/ours-q35-4b-joint-window10s-20260919/step
    \hline
    \multirow{2}{*}{Qwen3.5-9B} & \TSnoft & \cellcolor{gray!15}32.14 & \cellcolor{gray!15}58.17 & \cellcolor{gray!15}65.30 & \cellcolor{gray!15}2.08 & \cellcolor{gray!15}30.19 & \cellcolor{gray!15}56.64 & \cellcolor{gray!15}64.38 & \cellcolor{gray!15}11.24 & \cellcolor{gray!15}31.69 & \cellcolor{gray!15}61.09 & \cellcolor{gray!15}64.98 & \cellcolor{gray!15}11.10 & \cellcolor{gray!15}29.68 & \cellcolor{gray!15}51.08 & \cellcolor{gray!15}63.18 & \cellcolor{gray!15}10.57 \\ % DETAIL_SOURCE METRICS_CELL anchor2/q35-9b-recent10/phase anchor2/q35-9b-recent10/step anchor2/q35-9b-recent10/action anchor3/q35-9b-recent10/step
    {} & \TSyesft & \cellcolor{gray!15}72.37 & \cellcolor{gray!15}41.48 & \cellcolor{gray!15}66.52 & \cellcolor{gray!15}79.65 & \cellcolor{gray!15}61.57 & \cellcolor{gray!15}41.72 & \cellcolor{gray!15}66.92 & \cellcolor{gray!15}75.94 & \cellcolor{gray!15}49.19 & \cellcolor{gray!15}54.43 & \cellcolor{gray!15}67.77 & \cellcolor{gray!15}64.61 & \cellcolor{gray!15}48.43 & \cellcolor{gray!15}31.75 & \cellcolor{gray!15}58.98 & \cellcolor{gray!15}65.52 \\ % DETAIL_SOURCE METRICS_CELL anchor2/ours-q35-9b-recent10reset/phase anchor2/ours-q35-9b-recent10reset/step anchor2/ours-q35-9b-recent10reset/action anchor3/ours-q35-9b-recent10reset/step
    \noalign{\hrule height 1pt}
  \end{tabular}
  \end{adjustbox}
  \vspace{-0.2cm}
    \caption{Detailed metrics for the main results in Table~\ref{tab:main_results}.}
  \vspace{-0.2cm}
\label{tab:details_main_results}
\label{tab:details_hipropa_phase}
\label{tab:details_hipropa_step}
\label{tab:details_hipropa_action}
\label{tab:details_ego}
\end{table*}

\begin{table*}[h]
  \renewcommand{\cellcolor}[1]{} % Plain result cells; retain status markup for automatic updates.
  \centering
  \scriptsize
  \setlength{\tabcolsep}{1.5pt}
  \renewcommand{\arraystretch}{1.15}
  \begin{adjustbox}{max width=\linewidth}
  \begin{tabular}{@{}l@{}l|cccc|cccc@{}}
    \noalign{\hrule height 1pt}
    \multicolumn{2}{l|}{\multirow{2}{*}{Supervision}} & \multicolumn{4}{c|}{ProactiveCoachBench Step} & \multicolumn{4}{c}{EgoProactive} \\
    \cline{3-6}\cline{7-10}
    & & sPrecision & sRecall & Response F1 & Silence F1 & sPrecision & sRecall & Response F1 & Silence F1 \\
    \noalign{\hrule height 0.6pt}
    \multicolumn{10}{@{}l}{\textit{Qwen3-VL-4B}} \\
    {} & Step-only & \cellcolor{gray!15}40.72 & \cellcolor{gray!15}48.23 & \cellcolor{gray!15}66.87 & \cellcolor{gray!15}59.99 & \cellcolor{gray!15}50.61 & \cellcolor{gray!15}27.95 & \cellcolor{gray!15}55.10 & \cellcolor{gray!15}66.30 \\ % DETAIL_SOURCE SUPERVISION_STEP q3vl-4b checkpoint=939
    {} & Multi-level (Ours) & \cellcolor{gray!15}59.13 & \cellcolor{gray!15}44.45 & \cellcolor{gray!15}68.04 & \cellcolor{gray!15}75.30 & \cellcolor{gray!15}47.66 & \cellcolor{gray!15}31.86 & \cellcolor{gray!15}60.00 & \cellcolor{gray!15}65.69 \\ % DETAIL_SOURCE SUPERVISION_OURS q3vl-4b
    \hline
    \multicolumn{10}{@{}l}{\textit{Qwen3-VL-8B}} \\
    {} & Step-only & \cellcolor{gray!15}48.58 & \cellcolor{gray!15}46.09 & \cellcolor{gray!15}66.02 & \cellcolor{gray!15}66.22 & \cellcolor{gray!15}50.18 & \cellcolor{gray!15}28.67 & \cellcolor{gray!15}56.88 & \cellcolor{gray!15}67.09 \\ % DETAIL_SOURCE SUPERVISION_STEP q3vl-8b checkpoint=939
    {} & Multi-level (Ours) & \cellcolor{gray!15}58.70 & \cellcolor{gray!15}46.40 & \cellcolor{gray!15}69.05 & \cellcolor{gray!15}75.12 & \cellcolor{gray!15}50.38 & \cellcolor{gray!15}29.57 & \cellcolor{gray!15}58.78 & \cellcolor{gray!15}67.65 \\ % DETAIL_SOURCE SUPERVISION_OURS q3vl-8b
    \hline
    \multicolumn{10}{@{}l}{\textit{Qwen3.5-4B}} \\
    {} & Step-only & \cellcolor{gray!15}42.76 & \cellcolor{gray!15}41.77 & \cellcolor{gray!15}63.85 & \cellcolor{gray!15}65.22 & \cellcolor{gray!15}47.85 & \cellcolor{gray!15}30.92 & \cellcolor{gray!15}57.02 & \cellcolor{gray!15}64.42 \\ % DETAIL_SOURCE SUPERVISION_STEP q35-4b checkpoint=939 window10s source=table4_levels_eval_20260919
    {} & Multi-level (Ours) & \cellcolor{gray!15}59.73 & \cellcolor{gray!15}44.23 & \cellcolor{gray!15}69.02 & \cellcolor{gray!15}75.68 & \cellcolor{gray!15}48.56 & \cellcolor{gray!15}30.44 & \cellcolor{gray!15}56.32 & \cellcolor{gray!15}64.04 \\ % DETAIL_SOURCE SUPERVISION_OURS q35-4b checkpoint=939 window10s source=joint_window_q35-4b_20260919
    \hline
    \multicolumn{10}{@{}l}{\textit{Qwen3.5-9B}} \\
    {} & Step-only & \cellcolor{gray!15}44.82 & \cellcolor{gray!15}42.89 & \cellcolor{gray!15}63.77 & \cellcolor{gray!15}66.69 & \cellcolor{gray!15}51.17 & \cellcolor{gray!15}26.64 & \cellcolor{gray!15}53.07 & \cellcolor{gray!15}66.69 \\ % DETAIL_SOURCE SUPERVISION_STEP q35-9b
    {} & Multi-level (Ours) & \cellcolor{gray!15}61.57 & \cellcolor{gray!15}41.72 & \cellcolor{gray!15}66.92 & \cellcolor{gray!15}75.94 & \cellcolor{gray!15}48.43 & \cellcolor{gray!15}31.75 & \cellcolor{gray!15}58.98 & \cellcolor{gray!15}65.52 \\ % DETAIL_SOURCE SUPERVISION_OURS q35-9b
    \noalign{\hrule height 1pt}
  \end{tabular}
  \end{adjustbox}
  \vspace{-0.2cm}
\caption{Detailed metrics for hierarchical vs. step-only supervision in Table~\ref{tab:multilevel-supervision}.}
  \vspace{-0.3cm}
  \label{tab:details_multilevel_supervision}
\end{table*}

\begin{table*}[h]
  \renewcommand{\cellcolor}[1]{} % Plain result cells; retain status markup for automatic updates.
  \centering
  \scriptsize
  \setlength{\tabcolsep}{1.5pt}
  \renewcommand{\arraystretch}{1.15}
  \begin{adjustbox}{max width=\linewidth}
  \begin{tabular}{@{}l|cccc|cccc@{}}
    \noalign{\hrule height 1pt}
    \multirow{2}{*}{Supervision} & \multicolumn{4}{c|}{ProactiveCoachBench Step} & \multicolumn{4}{c}{EgoProactive} \\
    \cline{2-5}\cline{6-9}
    & sPrecision & sRecall & Response F1 & Silence F1 & sPrecision & sRecall & Response F1 & Silence F1 \\
    \noalign{\hrule height 0.6pt}
    step-only & \cellcolor{gray!15}42.76 & \cellcolor{gray!15}41.77 & \cellcolor{gray!15}63.85 & \cellcolor{gray!15}65.22 & \cellcolor{gray!15}47.85 & \cellcolor{gray!15}30.92 & \cellcolor{gray!15}57.02 & \cellcolor{gray!15}64.42 \\ % DETAIL_SOURCE LEVEL_SFT_COMPLETE step checkpoint=939 window10s source=table4_levels_eval_20260919
    phase-step & \cellcolor{gray!15}48.32 & \cellcolor{gray!15}51.12 & \cellcolor{gray!15}67.89 & \cellcolor{gray!15}64.59 & \cellcolor{gray!15}48.29 & \cellcolor{gray!15}29.26 & \cellcolor{gray!15}55.16 & \cellcolor{gray!15}64.39 \\ % DETAIL_SOURCE LEVEL_SFT_COMPLETE phase-step checkpoint=939 window10s source=table4_levels_eval_20260919
    step-action & \cellcolor{gray!15}56.57 & \cellcolor{gray!15}41.09 & \cellcolor{gray!15}66.56 & \cellcolor{gray!15}75.32 & \cellcolor{gray!15}45.60 & \cellcolor{gray!15}35.52 & \cellcolor{gray!15}61.19 & \cellcolor{gray!15}62.32 \\ % DETAIL_SOURCE LEVEL_SFT_COMPLETE step-action
    phase-step-action & \cellcolor{gray!15}59.73 & \cellcolor{gray!15}44.23 & \cellcolor{gray!15}69.02 & \cellcolor{gray!15}75.68 & \cellcolor{gray!15}48.56 & \cellcolor{gray!15}30.44 & \cellcolor{gray!15}56.32 & \cellcolor{gray!15}64.04 \\ % DETAIL_SOURCE LEVEL_SFT_COMPLETE phase-step-action checkpoint=939 window10s source=joint_window_q35-4b_20260919
    \noalign{\hrule height 1pt}
  \end{tabular}
  \end{adjustbox}
  \vspace{-0.2cm}
\caption{Detailed metrics for the supervision-level ablation in Table~\ref{tab:training-levels-ablation}.}
  \vspace{-0.3cm}
  \label{tab:details_training_levels}
\end{table*}

\begin{table*}[!h]
  \centering
  \scriptsize
  \setlength{\tabcolsep}{1.5pt}
  \renewcommand{\arraystretch}{1.15}
  \begin{adjustbox}{max width=\linewidth}
  \begin{tabular}{@{}c|cccc|cccc|cccc@{}}
    \noalign{\hrule height 1pt}
    \multirow{2}{*}{FT} & \multicolumn{4}{c|}{Phase} & \multicolumn{4}{c|}{Step} & \multicolumn{4}{c}{Action} \\
    \cline{2-5}\cline{6-9}\cline{10-13}
    & sPrecision & sRecall & Response F1 & Silence F1 & sPrecision & sRecall & Response F1 & Silence F1 & sPrecision & sRecall & Response F1 & Silence F1 \\
    \noalign{\hrule height 0.6pt}
    \TSnoft & 15.06 & 6.76 & 15.17 & 69.69 & 14.71 & 6.05 & 13.22 & 64.65 & 29.21 & 59.74 & 63.38 & 1.94 \\ % DETAIL_SOURCE JOINT_GUIDANCE zero-shot q35_4b_joint_zeroshot_20260923
    \TSyesft & 72.89 & 44.05 & 69.86 & 80.83 & 59.73 & 44.23 & 69.02 & 75.68 & 47.18 & 57.04 & 68.56 & 61.15 \\ % DETAIL_SOURCE JOINT_GUIDANCE ours q35_4b_joint_zeroshot_20260923
    \noalign{\hrule height 1pt}
  \end{tabular}
  \end{adjustbox}
  \vspace{-0.2cm}
  \caption{Detailed metrics for zero-shot multi-level guidance in Table~\ref{tab:joint-hierarchical-guidance}.}
  \vspace{-0.4cm}
  \label{tab:details_joint_guidance}
\end{table*}
