# Supplementary material for: Improving Proactive AI Assistance with Hierarchical Procedural Understanding
Source: arXiv:2610.06505 source file (2026-10-06)
Supplement: Supplementary file 6 [file d_evaluation_details.tex]

\section{Details of Evaluation Protocol}
\label{details of evaluation protocol}

\subsection{Training Configurations}
\label{training configurations}
Table~\ref{tab:sft_hyperparameters} summarizes the training settings.
We keep the original task instructions.
Video chunks and target outputs are ordered by time, with each output placed at its reference timestamp.
We used sliding-window causal attention, restricting direct access to video tokens from the latest five chunks (10 seconds), including the current chunk, while retaining task instructions and prior output text within the context limit.

\begin{table}[h]
  \centering
  \small
  \setlength{\tabcolsep}{5pt}
  \renewcommand{\arraystretch}{1.12}
  \begin{adjustbox}{max width=\textwidth}
  \begin{tabular}{lc}
    \toprule
    \textbf{Setting} & \textbf{Shared configuration} \\
    \midrule
    Training hardware & 8 NVIDIA B200 GPUs \\
    Optimizer & AdamW \\
    Learning rate & $2\times10^{-5}$ \\
    Learning-rate schedule & Cosine decay; 5\% warmup \\
    Weight decay & 0.1 \\
    Gradient clipping norm & 1.0 \\
    Training epochs & 3 \\
    Effective batch size & 32 sequences \\
    Maximum sequence length & 98,304 tokens \\
    Numerical precision & BF16 \\
    Distributed training & DeepSpeed ZeRO stage 1 \\
    Video sampling rate & 1 fps \\
    Video chunk & 2 frames \\
    \bottomrule
  \end{tabular}
  \end{adjustbox}
  \caption{Shared SFT configurations.}
  \label{tab:sft_hyperparameters}
\end{table}

%%% JSL %%%%
% \red{공통 SFT 설정은 Table~\ref{tab:sft_hyperparameters}에 정리한다.
% 영상은 1fps로 관측하여 두 프레임을 하나의 2초 청크로 구성하고,
% 원본 안내 문장과 참조 발화 시점을 유지한 채 영상과 정답 출력을 시간순으로 배치한다.
% Qwen3-VL-4B/8B의 Window SFT는 sliding-window causal attention을 사용하여
% 현재 청크를 포함한 최근 5개 청크(10초)의 영상 토큰에만 직접 접근하며,
% 작업 지시문과 이전 출력 텍스트는 문맥 길이 한도 내에서 유지한다.
% Qwen3.5-4B/9B는 full causal attention으로 학습한다.}
%%% JSL %%%%

\begingroup
\raggedbottom

\subsection{Evaluation Prompts}
\label{evaluation inputs and baseline prompts}
Figure~\ref{fig:evaluation-shared-input} shows the inputs shared by all baseline models: the task goal, the most recent 10 seconds of video, the ground-truth dialogue history, and the requested guidance level.
Frontier models and multimodal baselines, including Qwen, use the shared prompt in Figure~\ref{fig:evaluation-prompt-qwen35-zs}.
Figure~\ref{fig:evaluation-prompt-streaming} shows the prompts for streaming and proactive assistance models, and Figure~\ref{fig:evaluation-prompt-ours} shows the prompt for our model.


\begin{figure}[H]
\centering
\captionsetup{skip=4pt}
\begin{tcolorbox}[
colback=gray!3,
colframe=gray!50,
coltitle=black,
title={Common Inputs},
fonttitle=\small\bfseries,
fontupper=\footnotesize,
boxrule=0.5pt,
arc=1mm]

\textbf{Task Goal.}\par
\{task\_goal\}\par\smallskip

\textbf{Requested Guidance Level.}\par
\{Phase / Step / Action\}\par
Phase: a high-level unit that achieves an intermediate goal through multiple steps.\par
Step: a procedural unit that achieves a specific outcome through multiple actions.\par
Action: an observable fine-grained event that can be guided independently.\par\smallskip

\textbf{Ground-Truth Dialogue History.}\par
At \{past\_time\}s: \{past\_GT\_guidance\}\par
Additional ground-truth guidance strictly preceding the current anchor, if any.\par
Past guidance describes what was said, not proof of completion.\par\smallskip

\textbf{Current Observation.}\par
Current anchor: \{time\}s.\par
The most recent 10 seconds of video preceding the current anchor.

\end{tcolorbox}
\caption{Common inputs for evaluation.}
\label{fig:evaluation-shared-input}
\end{figure}

\begin{figure}[H]
\centering
\captionsetup{skip=4pt}
\begin{tcolorbox}[
colback=gray!3,
colframe=gray!50,
coltitle=black,
title={Frontier and Multimodal Baselines},
fonttitle=\small\bfseries,
fontupper=\footnotesize,
boxrule=0.5pt,
arc=1mm]

You are a proactive assistant helping a user perform a procedural task.
Use the current observation and ground-truth dialogue history to determine whether new guidance is needed at the requested guidance level.
If guidance is needed, provide one concise instruction that helps achieve the task goal.
Output one line: \texttt{\$interrupt\$} followed by the instruction, or \texttt{\$silent\$} when no new guidance is needed.\par\smallskip

Based on the current observation and previous guidance, determine whether new guidance is needed at the requested guidance level.
If needed, provide one concise instruction for the task.

\end{tcolorbox}
\caption{Shared evaluation prompt for frontier models and multimodal baselines, including Qwen.}
\label{fig:evaluation-prompt-qwen35-zs}
\end{figure}

\begin{figure}[H]
\centering
\captionsetup{skip=4pt}
\begin{tcolorbox}[
colback=gray!3,
colframe=gray!50,
coltitle=black,
title={Streaming and Proactive Assistance Models},
fonttitle=\small\bfseries,
fontupper=\footnotesize,
boxrule=0.5pt,
arc=1mm]

\textbf{\small VideoLLM-Online and ProAssist.}\par\smallskip
You are a proactive assistant helping a user perform a procedural task.
Use the current observation and previous guidance to determine whether new guidance is needed at the requested guidance level.
Use the native streaming gate to remain silent when no new guidance is needed.
When the gate selects a response, provide one concise instruction that helps achieve the task goal.\par\smallskip
Based on the current observation and previous guidance, determine whether new guidance is needed at the requested guidance level.
If needed, provide one concise instruction for the task.\par\medskip

\textbf{\small VideoChat3-4B.}\par\smallskip
You are a proactive visual assistant helping a user perform a procedural task.
Use the current observation and previous guidance to determine whether new guidance is needed at the requested guidance level.
If guidance is needed, output \texttt{\textless{}/Response\textgreater{}} followed by one concise instruction that helps achieve the task goal.
If no useful new guidance is needed, output \texttt{\textless{}/Silence\textgreater{}}.\par\smallskip
Based on the current observation and previous guidance, determine whether new guidance is needed at the requested guidance level.
If needed, provide one concise instruction for the task.\par\medskip

\textbf{\small MMDuet2.}\par\smallskip
You are a proactive assistant helping a user perform a procedural task.
Use the current observation and previous guidance to determine whether new guidance is needed at the requested guidance level.\par\smallskip
Based on the current observation and previous guidance, determine whether new guidance is needed at the requested guidance level.
If needed, provide one short imperative instruction for the task.
\end{tcolorbox}
\caption{Prompts for streaming and proactive assistance models.}
\label{fig:evaluation-prompt-streaming}
\end{figure}

\begin{figure}[H]
\centering
\captionsetup{skip=4pt}
\begin{tcolorbox}[
colback=gray!3,
colframe=gray!50,
coltitle=black,
title={Our Multi-Level Model},
fonttitle=\small\bfseries,
fontupper=\footnotesize,
boxrule=0.5pt,
arc=1mm]

You are a proactive procedural assistant watching a first-person video stream.
Use the goal, observed frames, and prior outputs to decide whether to guide.
Do not repeat a guide or guide an already finished unit.\par

Output exactly \texttt{\textless{}silent\textgreater{}} when no new guidance is needed.
Otherwise output \texttt{\textless{}response\textgreater{}} followed only by the guidance entries needed now, separated by `` / '':\par
\texttt{phase P: guidance / step P-S: guidance / action P-S-A: guidance}\par

Positive numbered IDs express parent--child relationships.
Number units in temporal order within the clip and restart child numbers under each parent.
Put entries in Phase, Step, Action order and omit inactive levels.

\end{tcolorbox}
\caption{Evaluation prompt for our model.}
\label{fig:evaluation-prompt-ours}
\end{figure}

\endgroup
