# Supplementary material for: Improving Proactive AI Assistance with Hierarchical Procedural Understanding
Source: arXiv:2610.06505 source file (2026-10-06)
Supplement: Supplementary file 7 [file dataset_storyboards.tex]

% Original dataset annotation storyboards; provenance in ThinkStream/paper_draft/dataset_storyboards_selected_20260925/.
\begingroup
\raggedbottom
\Needspace{.92\textheight}
\section{Examples of ProactiveCoachBench}
These six examples illustrate the hierarchically structured guidance in ProactiveCoachBench.
Red denotes the task goal, and blue shows phase-, step-, and action-level guidance at the first six consecutive guidance times.
\label{huppa examples}

\begin{figure}[H]
\centering
% Review sample H062; original record 35e43599-f438-4bc9-8983-68cecaf330e8
\includegraphics[width=\linewidth,height=.37\textheight,keepaspectratio]{figs/dataset_storyboard_01.pdf}
\caption{ProactiveCoachBench example-1 (goal: clean and lubricate a bicycle chain).}
\label{fig:dataset-storyboard-01}
\vspace{2cm}
% Review sample H064; original record 7ab371e9-704d-42d0-a130-217260e169ec
\includegraphics[width=\linewidth,height=.37\textheight,keepaspectratio]{figs/dataset_storyboard_02.pdf}
\caption{ProactiveCoachBench example-2 (goal: make a tossed vegetable salad).}
\label{fig:dataset-storyboard-02}
\end{figure}

% \clearpage
\begin{figure}[H]
\centering
% Review sample H083; original record z021-june-20-22-printer_big
\includegraphics[width=\linewidth,height=.40\textheight,keepaspectratio]{figs/dataset_storyboard_03.pdf}
\caption{ProactiveCoachBench example-3 (goal: replace a toner cartridge and load paper).}
\label{fig:dataset-storyboard-03}
\vspace{2cm}
% Review sample H086; original record z047-june-25-22-gladom_assemble
\includegraphics[width=\linewidth,height=.40\textheight,keepaspectratio]{figs/dataset_storyboard_04.pdf}
\caption{ProactiveCoachBench example-4 (goal: assemble a tray frame).}
\label{fig:dataset-storyboard-04}
\end{figure}

% \clearpage
\begin{figure}[H]
\centering
% Review sample H123; original record R160-3Oct-RAM
\includegraphics[width=\linewidth,height=.40\textheight,keepaspectratio]{figs/dataset_storyboard_05.pdf}
\caption{ProactiveCoachBench example-5 (goal: upgrade computer RAM and reconnect cables).}
\label{fig:dataset-storyboard-05}
\vspace{2cm}
% Review sample H154; original record z143-aug-17-22-nespresso
\includegraphics[width=\linewidth,height=.40\textheight,keepaspectratio]{figs/dataset_storyboard_06.pdf}
\caption{ProactiveCoachBench example-6 (goal: make a cup of coffee).}
\label{fig:dataset-storyboard-06}
% \vspace{0.7em}
\end{figure}

% \clearpage
\clearpage
\endgroup
