# Supplementary material for: Improving Proactive AI Assistance with Hierarchical Procedural Understanding
Source: arXiv:2610.06505 source file (2026-10-06)
Supplement: Supplementary file 8 [file e_metrics.tex]

\section{Details of Metrics}
\label{details of metrics}
We provide detailed descriptions of sF1, gF1, and PQS.
sF1 considers both the semantic alignment between generated and GT guidance and the coverage of GT guidance through temporal--semantic matching~\citep{guideme}.
gF1 considers both response F1 and silent F1 at anchor points.
PQS reflects the correctness of response--silence decisions and the quality of generated guidance~\citep{pwr}.
All metrics are computed independently for each dataset and guidance level.

\subsection{Soft F1 (sF1)}
\label{sf1}
Following GuideMe~\citep{guideme}, we partition each video at the midpoints $b_j=(\tau_j+\tau_{j+1})/2$ between consecutive GT response timestamps $\tau_j$ and $\tau_{j+1}$.
Within each segment, we perform minimum-cost one-to-one matching between predicted responses and GT anchors.
For a predicted response $(\hat y_i,t_i)$ and a GT response $(y_j,\tau_j)$, the semantic similarity $s_{ij}$ and matching cost $c_{ij}$ are
\begin{equation}
s_{ij}=\left|\cos\left(e(\hat y_i),e(y_j)\right)\right|,\qquad c_{ij}=(1-s_{ij})+\left[1-\exp\left(-0.01(t_i-\tau_j)^2\right)\right].
\label{eq:metric-matching-cost}
\end{equation}
Here, $e$ is the \texttt{all-mpnet-base-v2} sentence encoder, and timestamps are measured in seconds.
Since Silent Anchors contain no GT guidance, we set the semantic term $(1-s_{ij})$ to 1 when matching a predicted response to a Silent Anchor.
The final matching set $\mathcal M$ includes only pairs in which both the prediction and GT are responses.

sPrecision (sP) measures how well the generated responses semantically match the GT responses, while sRecall (sR) measures how completely the GT responses are covered.
Let $P$ and $R$ denote the numbers of predicted and GT responses, respectively, and $C$ the sum of semantic similarities over matched pairs.
We compute sPrecision and sRecall by dividing $C$ by $P$ and $R$, respectively, and sF1 as their harmonic mean:
\begin{equation}
C=\sum_{(i,j)\in\mathcal M}s_{ij},\qquad
\mathrm{sP}=\frac{C}{P},\qquad
\mathrm{sR}=\frac{C}{R},\qquad
\mathrm{sF1}=
\frac{2\,\mathrm{sP}\cdot\mathrm{sR}}{\mathrm{sP}+\mathrm{sR}}
=\frac{2C}{P+R}.
\label{eq:metric-sf1}
\end{equation}
We multiply sPrecision, sRecall, and sF1 by 100 when reporting results.
Predicted responses without a matched GT response lower sPrecision, while GT responses without a matched prediction lower sRecall.
The temporal cost affects the matching assignment but does not directly penalize the final sF1 score.

\subsection{G-Mean F1 (gF1)}
\label{g-mean f1 (gf1)}
gF1 is computed from response--silence decisions at the original anchors.
At a GT Response Anchor, a predicted response counts as TP and predicted silence as FN.
At a GT Silent Anchor, predicted silence counts as TN and a predicted response as FP.
Response F1 (RF1) treats response as the positive class and evaluates whether the model responds when guidance is needed.
Silent F1 (SF1) treats silence as the positive class and evaluates whether the model remains silent when guidance is not needed.
Following PWR~\citep{pwr}, we compute gF1 as the geometric mean of these two scores:
\begin{equation}
\mathrm{RF1}=\frac{2\mathrm{TP}}{2\mathrm{TP}+\mathrm{FP}+\mathrm{FN}},\qquad \mathrm{SF1}=\frac{2\mathrm{TN}}{2\mathrm{TN}+\mathrm{FP}+\mathrm{FN}},\qquad \mathrm{gF1}
=100\,\sqrt{\mathrm{RF1}\cdot\mathrm{SF1}}.
\label{eq:metric-gmean-f1}
\end{equation}
gF1 does not use temporal matching or assess response content; an inaccurate response at a GT Response Anchor still counts as TP.

\subsection{Proactive Assistance Quality Score (PQS)}
\label{proactive assistance quality score (pqs)}
PQS jointly evaluates decision correctness and response quality at the original anchors.
For each TP response, GPT-5.2 evaluates the generated guidance against the GT guidance using the evaluation prompt and scoring rubric from PWR~\citep{pwr}.
The judge assigns ratings $r_{i,d}\in{1,\ldots,5}$ for relevance, specificity, actionability, and conciseness.
We normalize the mean rating to a content score $g_i\in[0,1]$ and compute PQS as
\begin{equation}
\bar r_i=\frac{1}{4}\sum_{d=1}^{4}r_{i,d},\qquad g_i=\frac{\bar r_i-1}{4},\qquad \mathrm{PQS}=\frac{100}{N}\left(\mathrm{TN}+\sum_{i\in\mathcal T}g_i\right).
\label{eq:metric-pqs}
\end{equation}
Here, $\mathcal T$ is the set of TP responses, and $N=\mathrm{TP}+\mathrm{TN}+\mathrm{FP}+\mathrm{FN}$ is the total number of anchors.
Each anchor receives a score of 1 for TN (correct silence), $g_i$ for a TP response, and 0 for FP or FN.
The final score is the average over all anchors, multiplied by 100.
On ProactiveCoachBench, which contains equal numbers of Response and Silent Anchors, an always-silent predictor obtains a PQS of 50 but a gF1 of 0.
We therefore interpret PQS alongside gF1.
