# Supplementary material for: Improving Proactive AI Assistance with Hierarchical Procedural Understanding
Source: arXiv:2610.06505 source file (2026-10-06)
Supplement: Supplementary file 9 [file f_additional_quantitative_results.tex]

% Appendix F. Active quantitative results from e_additional_results.tex.
\section{Additional Quantitative Results}
\vspace{-0.3cm}
\label{additional quantitative results}
\input{sec/appendix/d_detailed_metrics}

% Earlier commented experiments and writing notes remain in
% sec/appendix/e_additional_results.tex (not included in the paper).
