# Supplementary material for: Improving Proactive AI Assistance with Hierarchical Procedural Understanding
Source: arXiv:2610.06505 source file (2026-10-06)
Supplement: Supplementary file 10 [file g_qualitative_results.tex]

\section{Qualitative Results}
\vspace{-0.3cm}
\label{qualitative results}
Figures~\ref{fig:anchor-qualitative-01}--\ref{fig:anchor-qualitative-06} present six qualitative examples from ProactiveCoachBench and EgoProactive.
Compared with the baselines, our model more consistently provides appropriate guidance at response anchors while remaining silent at silent anchors.
Its responses are also generally well aligned with the ground-truth guidance.

\begin{figure}[p]
\centering
\includegraphics[
width=\linewidth,
height=.40\textheight,
keepaspectratio
]{figs/fig_qualitative_example_01.pdf}
\caption{Qualitative comparison on ProactiveCoachBench-1 (goal: make a peanut butter and jelly tortilla roll).}
\label{fig:anchor-qualitative-01}


\vspace{0.5cm}

\includegraphics[
    width=\linewidth,
    height=.40\textheight,
    keepaspectratio
]{figs/fig_qualitative_example_02.pdf}
\caption{Qualitative comparison on ProactiveCoachBench-2 (goal: disassemble and clean a bicycle seat stay assembly).}
\label{fig:anchor-qualitative-02}


\end{figure}

\clearpage
\begin{figure}[p]
\centering
\includegraphics[
width=\linewidth,
height=.40\textheight,
keepaspectratio
]{figs/fig_qualitative_example_03.pdf}
\caption{Qualitative comparison on ProactiveCoachBench-3 (goal: remove dry sticks from a fence).}
\label{fig:anchor-qualitative-03}

\vspace{0.5cm}

\includegraphics[
    width=\linewidth,
    height=.40\textheight,
    keepaspectratio
]{figs/fig_qualitative_example_04.pdf}
\caption{Qualitative comparison on ProactiveCoachBench-4 (goal: perform a COVID-19 rapid antigen test).}
\label{fig:anchor-qualitative-04}


\end{figure}

\clearpage
\begin{figure}[p]
\centering
\includegraphics[
width=\linewidth,
height=.40\textheight,
keepaspectratio
]{figs/fig_qualitative_example_05.pdf}
\caption{Qualitative comparison on EgoProactive-5 (goal: clean ceiling fan blades).}
\label{fig:anchor-qualitative-05}


\vspace{0.5cm}

\includegraphics[
    width=\linewidth,
    height=.40\textheight,
    keepaspectratio
]{figs/fig_qualitative_example_06.pdf}
\caption{Qualitative comparison on EgoProactive-6 (goal: put a harness on a dog).}
\label{fig:anchor-qualitative-06}


\end{figure}
\clearpage
