# Supplementary material for: Improving Proactive AI Assistance with Hierarchical Procedural Understanding
Source: arXiv:2610.06505 source file (2026-10-06)
Supplement: Supplementary file 11 [file h_limitations.tex]

% Appendix H. Content preserved from g_limitations_release.tex.
\section{Limitations}
\label{limitations}
Our evaluation uses ground-truth dialogue history rather than model-generated outputs. When the model uses its own output history, further evaluation is needed to assess error accumulation and its ability to revise plans. In addition, guidance-level adaptation focuses on user-requested changes. Further research could explore how to infer the user’s expertise and understanding to adjust the guidance level automatically, potentially making assistance more useful in real-world interactions. Also, since some activities can be performed in different orders to achieve the same goal, evaluation methods that consider these alternatives are needed. Future work should extend training and evaluation to support long-term task tracking and plan revision, personalized guidance, and multiple valid execution orders.
